# Supplementary material for: A polariton electric field sensor
Source: arXiv:2004.04791 source file (2020-04-09)
Supplement: Supplementary file 1 [file efieldSensor_SM.pdf]

# Supplemental Material:
# A polariton electric field sensor

Emre Togan,[1] Yufan Li,[1] Stefan Faelt,[1,2] Werner Wegscheider,[2] and Atac Imamoglu[1]

[1]*Institute of Quantum Electronics, ETH Zurich, CH-8093 Zurich, Switzerland*

[2]*Solid State Physics Laboratory, ETH Zurich, CH-8093 Zurich, Switzerland*

**Contents**

**I. Detailed information on the optical & electrical measurement setup and the sample structure** 1

**II. Estimate of the sensitivity limited by shot noise** 3

**III. Influence of additional noise sources on sensitivity** 3

**IV. Estimate of change in electric potential due to photocurrent** 6

**V. Measurement of electric field sensitivity of 0.12 V-m$^{-1}$-Hz$^{-1/2}$** 8

**VI. Changes in the measured polariton linewidth with $V_{\mathrm{DC}}$ and its influence on sensitivity** 8

## I. DETAILED INFORMATION ON THE OPTICAL & ELECTRICAL MEASUREMENT SETUP AND THE SAMPLE STRUCTURE

A detailed schematic and description of the optical and electrical measurement setup is presented in Supplemental Figure 1 and its caption.

Our MBE grown sample contains a single $In_{0.04}Ga_{0.96}As$ coupled quantum well (QW) structure that is placed at an anti-node of a planar optical cavity. The mirrors of the optical cavity are two distributed brag reflectors (DBRs). The top (bottom) DBR mirror consist of alternating layers of 20 (25) pairs of AlAs and GaAs. The coupled QW structure is inside a *p*-*i*-*n* structure with *p*-*n* layer separation of 500 nm. The *p* and *n* layers are placed at nodes of the cavity field. The *p* layer is 40 nm thick and the *n* layer is 30 nm thick.

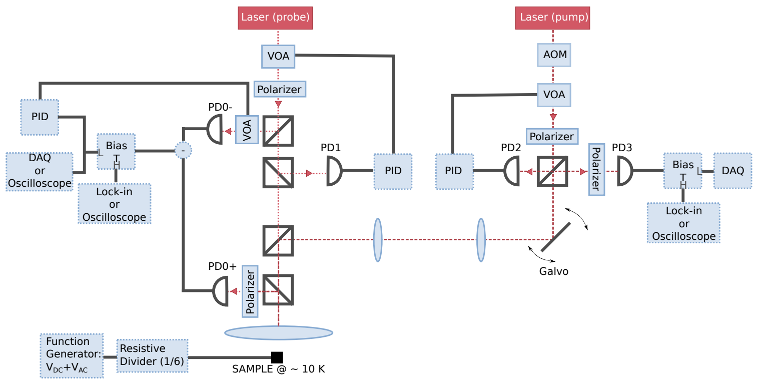


Supplemental Figure 1: Detailed schematic of the experimental setup. AC and DC voltages used to carry out the experiments are supplied by a function generator. We use a cryogenic resistive divider (1/6) to attenuate the output of function generator. The optical experiments use two lasers: the probe is an external cavity diode laser (New Focus Velocity TLB-6716) whereas the pump is a Ti:Saph laser (M Squared SolsTis). Both are intensity stabilized using PID control loops that stabilize the measured power (at PD1 or PD2) by varying the control voltage of a fiber optics based Variable Optical Attenuator (VOA). To be able to distinctly detect the reflected power of the two lasers at PD0+ and PD3 the two lasers are linearly orthogonally polarized using polarizers. Most of the reflected power of the probe laser (using a 10/90 beam splitter) is fiber coupled and sent to the + input of a biased photodiode (Thorlabs PDA450A, + input denoted PD0+ on the diagram). For all of the data in the main text and the supplemental material, with the exception of Supplemental Figure 2, the PD0- input of the same detector is blocked. The resulting signal is amplified and sent to a bias-T to separate the low and high frequency components, this separation allows the simultaneous recording of the mean reflected power as well as the oscillating optical power which gives us the $\Delta R$ signal. For $V_{\mathrm{AC}}$ at 76.226 kHz, $\Delta R$ is determined via a lock-in (SRS SR830). The lock-in time constant is 10 $\mu$s, the resulting signal is filtered with a 24 db/oct output filter. The filtered output of the lock-in is digitized at 100 k Samples/s and recorded simultaneously with the low-frequency reflection signal on the DAQ. For higher frequency measurements $>$ 100 kHz we digitize both the low and high frequency outputs of the bias-T on two seperate channels using a deep memory oscilloscope (Teledyne T3DS01102) and $\Delta R$ is determined via Fourier analysis of the recorded waveform. For the balanced detection in Supplemental Figure 2 to remove any common mode noise, the mean power detected on PD0+ and PD0- should be the same. We use an additional control loop (consisting of a VOA and PID keeping the mean difference signal to be zero) and rely on the limited bandwidth ($<$ 1 kHz) of the VOA to detect higher frequencies unimpeded by the control loop. The resulting amplified difference signal is treated the same way the PD0+ signal described before. For the pump laser we use a galvo mirror (Thorlabs GVS012) in the 4-f configuration to focus the pump laser to a variable spot on the sample. The reflected signal is fiber coupled and detected using a fast Avalanche Photo Diode (APD) denoted PD3 (Thorlabs APD130A), the output of which also is also split to low and high frequency components using a bias T and the high and low frequency components are digitized using a similar method. For the time traces presented in Figure 4 (main text) we record the power detected at locations indicated by PD0+ and PD3 using the APD130A directly connected to the the oscilloscope (without a bias-T). For these experiments recording time traces, different traces are recorded sequentially.

## II. ESTIMATE OF THE SENSITIVITY LIMITED BY SHOT NOISE

We estimate the expected sensitivity of a linear polariton electric field sensor by estimating the changes in the reflected power for a small electric field $E$ and assuming the standard deviation of the signal is determined solely by shot noise. We model the detected reflected power as a single Lorentzian:

$$R(\Delta) = P\left[1 - C\frac{(\Gamma/2)^2}{(\Delta - edE)^2 + (\Gamma/2)^2}\right]$$

Where $P$ is the mean detected power in photons per second, $\Gamma$ the FWHM polariton linewidth, $\Delta$ detuning of the laser from the polariton resonance, $ed$ is the dipole moment of the polariton, $C$ is the contrast of the polariton resonance in reflection and $E$ is the electric field to be sensed. We assume $edE \ll \Gamma$ and $\Delta = \pm\Gamma/2$. The reflected power (in photons/s) at this detuning is :

$$R(\pm\Gamma/2) \simeq P\left[1 - \frac{C}{2} \pm \frac{CedE}{\Gamma}\right]$$

When integrated for time $\tau$ the $\Delta R$ signal is $\pm P\tau\frac{CedE}{\Gamma}$. The standard deviation of this signal is determined by the mean detected photon number; assuming $\frac{CedE}{\Gamma} \ll (1 - C/2)$, the standard deviation of the signal for integration time $\tau$ is given by : $\sqrt{P\tau\,(1 - C/2)}$. We equate the signal to the standard deviation to find the electric field ($\delta E$) that can be detected with a signal to noise ratio of 1 under these conditions: $\delta E = \frac{\Gamma}{CPedT}\sqrt{P\tau\,(1 - C/2)} = \frac{\Gamma}{Ced}\sqrt{\frac{1-C/2}{\tau P}}$. The sensitivity ($\eta$) is related to $\delta E$ by : $\eta/\sqrt{\tau} = \delta E$. These two expressions yield Eq. (1) in the main text when solved for $\eta$.

## III. INFLUENCE OF ADDITIONAL NOISE SOURCES ON SENSITIVITY

In this section we illustrate presence of noise with different correlation times, and their effects on our measurements. We use the combined detector and intensity shot noise as a baseline, and refer to noise in excess of this level as excess noise. Supplemental Figure 2(a) illustrates the power dependence of this baseline; we plot the integrated average (RMS) voltage (measured at the output of the amplified photodetector, i.e. proportional to the detected power) as a function of laser power in the 1.7 - 1.8 MHz band for the reflected power off the sample for a laser energy that is detuned to the far red of the polariton resonances. The power dependence (green trace) shows the expected $\sqrt{A^2 + B^2P}$ where $P$ is the optical power on the detector, $A$ characterizes the detector noise and $B$ the relative strength of shot-noise. To verify that the measured level of $B$ is consistent with shot-noise we carry out a second experiment where the average voltage in the 1.7 to 1.8 MHz band from

the balanced output of the photodiode is plotted as a function of the detected power (red trace). Consistent with shot noise, the fit shows shows that $B$ value for the balanced detection is $\sqrt{2}$ times higher than the fit for a single detector. Since shot noise is independent (and equal in magnitude) for the + and - inputs of the balanced detector, we expect shot noise to add in quadrature, thus $B$ value should be higher by a factor of $\sqrt{2}$. We note that the balanced detection scheme reduces the structured noise that is present $< 500$ kHz (data not shown). This measurement establishes that the detected intensity noise around 1.75 MHz is determined by shot-noise and detector noise within the measurement range of 0 to 80 $\mu$W.

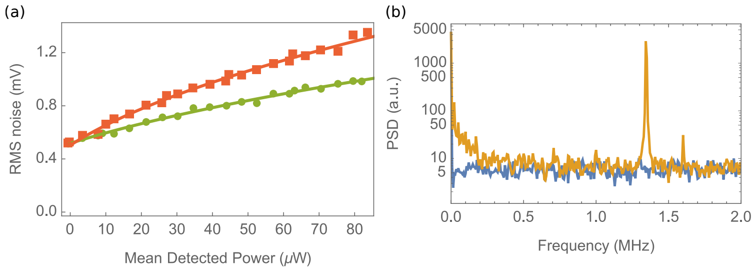


Supplemental Figure 2: (a) At a large detuning (laser to the red of polariton resonances) the integrated noise in the 1.7-1.8 MHz band over a 1.4 ms integration time for different mean powers detected on PD0+. The red curve is with PD0- unblocked (balanced detection) and green curve is with PD0- blocked (unbalanced detection). The solid lines are a fit to $\sqrt{A^2 + B^2 P}$, with $P$ the detected power, and we find the fit value for $B$ is a factor of $\sqrt{2}$ higher for the balanced detection compared to the unbalanced detection. (b) At 36 $\mu$W of detected power at PD0-, Power Spectral Density (PSD) obtained by taking the absolute square of the FFT of the recorded voltage waveform for a record of 14 ms. Data is recorded with 1.35 MHz 2 mVp-p $V_{\mathrm{AC}}$ at the point with highest $|\Delta R|$ (orange) or at a large red detuning (laser 200 $\mu$eV to the red of the polariton resonance) (blue). The detected signal at modulation frequency is clearly visible in the orange trace. The orange trace also exhibits strong noise at low frequencies and is overall higher in terms of the noise level, indicating at these high power levels the noise measured at a detuning that is sensitive to changes in the electric field exhibits more noise compared to the intensity noise of the reflected laser power. Low frequency PSD also shows peaks at particular frequencies, we pick the 76.226 kHz to fall into a minimum in this noise spectrum. (b)

The typical Power Spectral Density (PSD) of the detected signal is illustrated in Supplemental Figure 2(b). In blue is the baseline measurement with 37 $\mu$W of detected power, measured at a laser energy that is tuned to the far red of the polariton resonance. The yellow trace is acquired at the point with maximal $|\Delta R|$ with $V_{\mathrm{AC}} = 2$ mVp-p at 1.345349 MHz, with the same detected power. The AC modulation frequency is clearly visible in the yellow trace and is absent in the blue trace. The overall level of the yellow trace is higher compared to blue trace for almost all

frequencies, with the exception of the window around 1.75 MHz. There is also a marked difference at low frequencies between the two curves.

The presence of excess noise at the $V_{\rm AC}$ frequency increases the standard deviation of $\Delta R$ measured, hence decreases the sensitivity that is achievable. We work with AC frequencies that have little excess noise. For the high power measurements we work at 1.750181 MHz which falls in the window outlined previously, and at low powers we work at 76.226 kHz which again falls into a low excess noise region in the structured noise. We note that at the lower power of 200 nW, there is very little difference in the measured noise between the baseline measurement at large detuning and detuning with maximal $|\Delta R|$ at 76.226 kHz (data not shown).

Finally the low frequency noise also influences the measured standard deviation of $\Delta R$ at other frequencies: the $\Delta R$ value is extremely sensitive to the laser detuning, hence any fluctuation of the detuning leads to additional variations of $\Delta R$. We illustrate this in Supplemental Figure 3(b) where the time trace of $\Delta R$ with integration time $\tau = 5$ ms is plotted. The far detuned trace (yellow) shows the typical, measurement limited, variation of the data, and the green trace measured at maximal $\Delta R$ shows additional, slow, variations in addition to the variation shown on the yellow trace. At maximal $\Delta R$ the first order detuning dependence of $\Delta R$ is zero, but the trace still shows slow variation of $\Delta R$. On the polariton resonance (red trace) the detuning dependence of $\Delta R$ is first order and the red trace shows significant changes in the measured value of $\Delta R$. These time correlated changes in $\Delta R$ we attribute to low frequency noise in our setup (either electrical or mechanical) that leads to variation of the laser detuning, hence variations in $\Delta R$. This leads to an increase in the standard deviation of $\Delta R$ measured in the main text above the level expected from shot noise and detector noise.

These slow changes of $\Delta R$ also influence how the standard deviation of $\Delta R$ scales with the integration time $\tau$. These experiments were measured at low power (200 nW) and with $V_{\rm AC} = 2$ mVp-p at 76.226 kHz. To obtain the standard deviation vs $\tau$ plot for each trace, for each detuning we use a single dataset sampled at 100 kSamples/s. For different $\tau$ values we partition the data into non overlapping blocks of duration $\tau$ and take the mean of $\Delta R$ for each such duration. Standard deviation of different blocks is the standard deviation of $\Delta R$ for $\tau$. For a process that yields random, uncorrelated, values of $\Delta R$ with a fixed mean we expect the standard deviation of a measurement to scale as $\tau^{-1/2}$ where $\tau$ is the integration time used in the measurement. As Supplemental Figure 3(c) illustrates if the slow variations are significant in a time trace of $\Delta R$ the standard deviation of $\Delta R$ vs $\tau$ also diverges from the expected $\tau^{-1/2}$ behaviour.

For most of the experiments that we present in the text, the influence of this effect is relatively

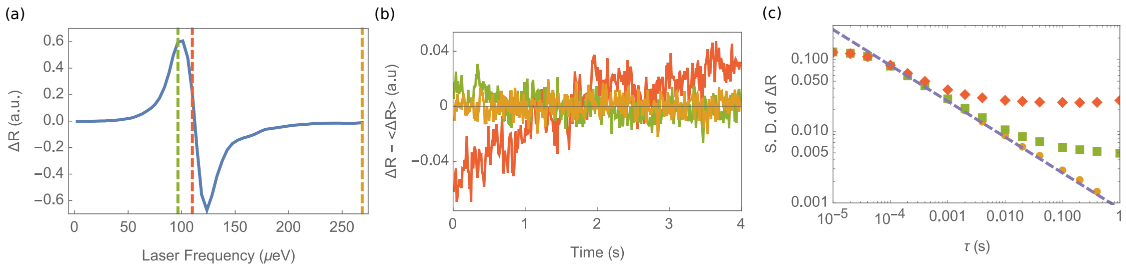


Supplemental Figure 3: (a) A plot of $\Delta R$ with $V_{\mathrm{DC}} = 8.9$ V vs laser frequency at the same position on the sample and under the same conditions to the data shown in Figure 2(a) (200 nW of laser power). The data is acquired for 4 s at 100 kSamples/s. Colors indicate the frequencies used to display the time traces of $\Delta R$ in panel (b), and to calculate standard deviation of $\Delta R$ vs $\tau$ in panel (c). (b) Time trace of $\Delta R$ (mean over the 4 s range is subtracted for clarity) at frequencies indicated in panel (a). The data is combined into non-overlapping 5 ms intervals, and the mean $\Delta R$ value for those 5 ms intervals are plotted. Time dependent changes in the value of $\Delta R$ are visible. (c) Standard deviation of $\Delta R$ vs $\tau$. For all detunings there is an initial plateau for short times caused by the finite time response introduced by the lock-in's output filter. Far detuned (yellow) data points follow the expected $\tau^{-1/2}$ behaviour, while both the red and green data points diverge from the $\tau^{-1/2}$ behaviour for times longer than 1 ms.

small, and becomes more significant when $\Delta R$ is more sensitive to changes in the laser detuning. We illustrate this in Supplemental Figure 4, in which the $\Delta R$ signal is measured with $V_{\mathrm{DC}} = 9.4$ V over 4 s intervals. We show the change in the standard deviation of $\Delta R$ as a function of the integration time for different laser frequencies. As illustrated in the figure, at the detuning that yields the minimal $\Delta R$ value (green data points) as well as when the laser is far detuned to the red of the polariton transition (yellow data points), the standard deviation of $\Delta R$ scales as $\tau^{-1/2}$. When the laser is tuned directly on the polariton resonance (red curve) the data diverges from this expected behaviour.

## IV. ESTIMATE OF CHANGE IN ELECTRIC POTENTIAL DUE TO PHOTOCURRENT

To estimate the effect of photocurrent on the potential at spatial locations far from the pump spot we carry out a 3D simulation of electric currents in a commericial finite element method simulator (COMSOL). We model the effect of the photocurrent produced by the pump laser as a point current source located at the origin of the simulation domain that injects $+I_{\mathrm{ph}}$ to the $n$ doped layer and $-I_{\mathrm{ph}}$ to the $p$ doped layer. We model the $p$ and $n$ doped layers as 40 nm and 30 nm thin resistive layers with respective conductivities of 30 kS m$^{-1}$ and 50 kS m$^{-1}$. These conductivites are based on room temperature transmission line measurements (also called transfer

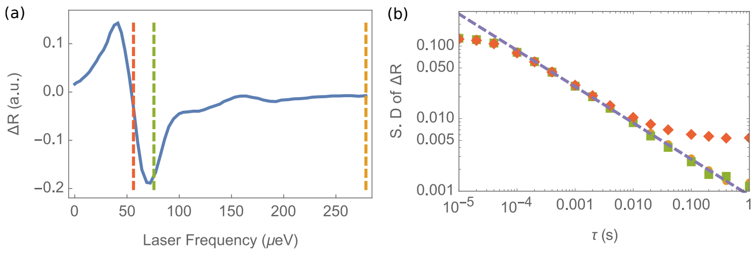


Supplemental Figure 4: (a) A plot of $\Delta R$ vs laser frequency with $V_{\mathrm{DC}} = 9.4$ V at the same position on the sample and under the same conditions to the data shown in Figure 2(a) (200 nW of laser power). For convenience we set 1.46041 eV as 0 eV. The data is acquired for 4 s at 100 kSamples/s. (b) Change of the standard deviation of $\Delta R$ as $\tau$ is varied. We calculate this for three seperate detunings denoted with dashed lines in (a). $\tau$ is equivalent to the time constant for lock-ins, or equivalently the integration time for the experiment. At higher $\tau$ values, for far red detuning (orange) and for minimal $\Delta R$ (green), the standard deviation follows the expected $\tau^{-1/2}$ scaling, indicating the noise is independent and random for each of the partitioned blocks. At the detuning that the $\Delta R$ signal has the highest derivative (red) the standard deviation diverges from the $\tau^{-1/2}$ scaling for $\tau > 5$ ms.

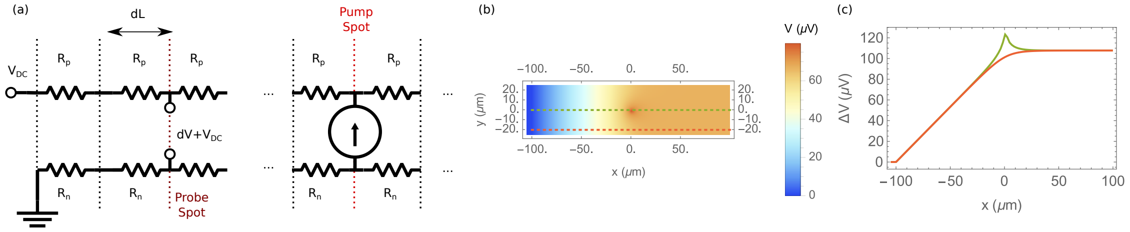


Supplemental Figure 5: (a) Schematic circuit diagram of the $p$ and $n$ layers with the applied potential and a current source modeling the photocurrent from the pump laser. We show discrete circuit elements for a distance dL, where the resistive doped layers are represented by resistors with resistances $R_p$ and $R_n$. The pump spot is modeled as a point current source. The change in the potential $dV$ at the probe spot (a different point in the sample) is then calculated as the potential difference between the $n$ and $p$ layers. (b) The potential distribution with a 50 nA current source at the origin for a 50 $\mu$m x 200 $\mu$m simulation area. (c) Line cuts (colors indicate the position of the line cuts in (b)) showing the potential difference between the $p$ and $n$ layers that forms due to the presence of the point current source.

length measurements) that yield sheet resistance of 800 $\Omega$/Sq and 600 $\Omega$/Sq for the $p$ and $n$ doped layers respectively (data not shown). A sketch of the equivalent circuit considered is illustrated in Supplementary Figure 5(a). We consider a rectangular geometry with an aspect ratio of 1:4 to highlight the role of constriction of the current on the developed potential. The potential of the two doped layers is fixed on the left hand side (for the illustration to 0 V), modeling the metal contacts on the sample, and the change in the potential due to the current is simulated. The spatial

distribution of the change of the potential in the $p$ doped layer is illustrated in Supplementery Figure 5(b). Supplementary Figure 5(c) show line cuts of the change in the potential between the two doped layers for two different values of $y$ (0 $\mu$m and -20 $\mu$m). As these figures illustrate presence of a 50 nA current (that is consistent with our measurements – data not shown), can generate a change in the potential as much as 110 $\mu$V, thus an electric field upto 0.2 kV/m in the simplified geometry considered. The resulting spatial profile is vastly different from the expected electric field distribution for charges or dipoles, and the current has an extremely long range influence. The figure illustrates that the resulting potential distribution depends on the geometry of the sample, where the metal contacts are deposited, any constrictions on the sample, etc. We note that this explanation is supportive of the long-range influence of excitation of polaritons at the pump spot, but further experiments need to be performed to exactly identify the photocurrent as the mechanism. We further note that, in addition to the peculiar spatial dependence, one expects to have a finite response time due to the capacitance that is present in the $p$-$i$-$n$ diode structure.

## V. MEASUREMENT OF ELECTRIC FIELD SENSITIVITY OF 0.12 V-M$^{-1}$-HZ$^{-1/2}$

The best measured sensitivity is illustrated in Supplemental Figure 6. We also show the power dependence of the $\Delta R$ signal, the power dependence of its standard deviation as well as the power dependence of sensitivity at $V_{\mathrm{DC}} = 9.1$ V.

## VI. CHANGES IN THE MEASURED POLARITON LINEWIDTH WITH $V_{\mathrm{DC}}$ AND ITS INFLUENCE ON SENSITIVITY

Changes in the lower polariton linewidth with $V_{\mathrm{DC}}$ and estimates of its influence on the sensitivity is shown in Supplemental Figure 7.

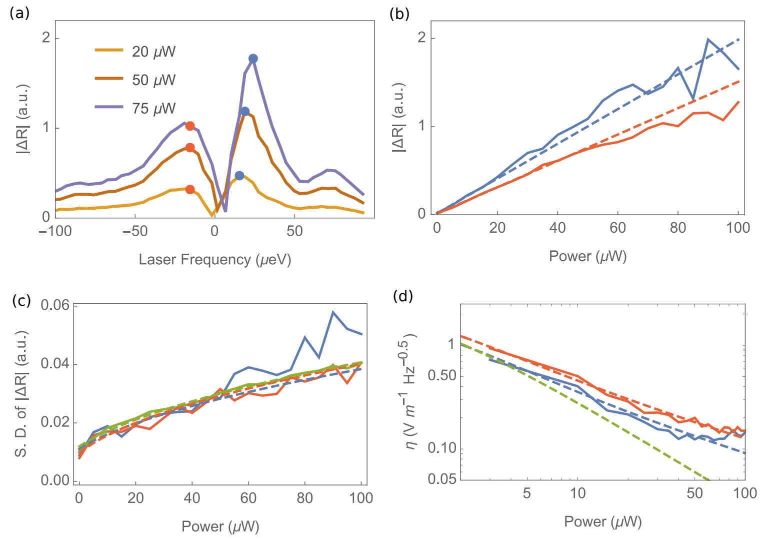


Supplemental Figure 6: Measurement of the best sensitivity. Similar to Figure 3 of the main text at a different spatial location with a similar cavity energy at $V_{\mathrm{DC}} = 9.1$ V. The best measured sensitivity is 0.12 V-m$^{-1}$-Hz$^{-1/2}$. In plots of laser detuning vs $|\Delta R|$ another peak (at high power) is visible at 75 $\mu$eV laser frequency which indicates the presence of photonic disorder in the system.

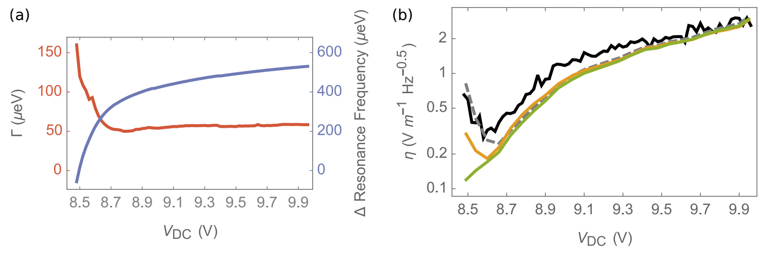


Supplemental Figure 7: Change of polariton linewidth with $V_{\mathrm{DC}}$ and its effect on sensitivity. (a) Change in the polariton linewidth and polariton transition frequency as a function of $V_{\mathrm{DC}}$ extracted from the data presented in Figure 1(c). The linewidth has a minimum of $\sim 50$ $\mu$eV at 8.7 V. (b) Sensitivity as a function of $V_{\mathrm{DC}}$, black and gray dashed lines are the same as Figure 2(b). We plot equation (1) in two additional traces. For the yellow trace, all parameters of the equation are the same as the gray dashed line except we set $\Gamma = 60$ $\mu$eV independent of $V_{\mathrm{DC}}$; for the green trace all parameters are same except $C = 0.8$. The yellow curve retains most of the features of the gray dashed line, however it predicts a better sensitivity than what is measured. The green curve predicts better sensitivites at lower $V_{\mathrm{DC}}$.
